# Supplementary material for: Optimizing Sequential Recommendation Models with Scaling Laws and Approximate Entropy
Source: arXiv:2412.00430 source file (2025-02-19)
Supplement: Supplementary file 1 [file chapterA_Appendix.tex]

\section{Appendix / supplemental material}
